# Supplementary material for: Noise-aware few-shot learning through bi-directional multi-view prompt alignment
Source: arXiv:2603.11617 source file (2026-03-12)
Supplement: Supplementary file 1 [file X_suppl.tex]

\clearpage
\setcounter{page}{1}
\maketitlesupplementary

% \usepackage{algorithm}
% \usepackage{algpseudocode} 
% \usepackage{algorithmicx}
% \usepackage{algorithmic}

% \section{Rationale}
% \label{sec:rationale}
% % 
% Having the supplementary compiled together with the main paper means that:
% % 
% \begin{itemize}
% \item The supplementary can back-reference sections of the main paper, for example, we can refer to \cref{sec:intro};
% \item The main paper can forward reference sub-sections within the supplementary explicitly (e.g. referring to a particular experiment); 
% \item When submitted to arXiv, the supplementary will already included at the end of the paper.
% \end{itemize}
% % 
% To split the supplementary pages from the main paper, you can use \href{https://support.apple.com/en-ca/guide/preview/prvw11793/mac#:~:text=Delete%20a%20page%20from%20a,or%20choose%20Edit%20%3E%20Delete).}{Preview (on macOS)}, \href{https://www.adobe.com/acrobat/how-to/delete-pages-from-pdf.html#:~:text=Choose%20%E2%80%9CTools%E2%80%9D%20%3E%20%E2%80%9COrganize,or%20pages%20from%20the%20file.}{Adobe Acrobat} (on all OSs), as well as \href{https://superuser.com/questions/517986/is-it-possible-to-delete-some-pages-of-a-pdf-document}{command line tools}.

\section{Method Details}
% \subsection{Method Details}
\paragraph{Training process}
We detail the training process of NA-MVP in Algorithm~\ref{alg:NA-MVP}, which includes a supervised phase and a denoising phase.

\paragraph{Optimal Transport}
OT is a powerful framework for mapping one probability distribution to another while minimizing the associated transportation cost. Given two distributions \( \boldsymbol{\mu} \in \mathbb{R}^m_+ \) and \( \boldsymbol{\nu} \in \mathbb{R}^n_+ \), and a cost matrix \( \boldsymbol{C} \in \mathbb{R}^{m \times n} \), the OT problem aims to find the optimal transport plan \( \boldsymbol{T} \) that minimizes the following objective:
%\vspace{-0.1cm}
\begin{gather}
d_{\text{OT}}(\mu, \nu) =\min_{\boldsymbol{T} \in \Pi(\boldsymbol{\mu}, \boldsymbol{\nu})} \langle \boldsymbol{C}, \boldsymbol{T} \rangle
\\
\Pi(\mu, \nu) = \left\{ \mathbf{T} \in \mathbb{R}_+^{m \times n} \;\middle|\; \mathbf{T} \mathds{1}_n = \mu, \; \mathbf{T}^\top \mathds{1}_m = \nu \right\}
\end{gather}
%\vspace{-0.1cm}
where \( \langle \cdot, \cdot \rangle \) represents the Frobenius dot-product, and \( \mathds{1}_m \), \( \mathds{1}_n \) denote the vectors of ones of length \( m \) and \( n \), respectively. Since solving OT exactly is computationally expensive, the entropy-regularized version is often used:
\begin{equation}
d_{\text{OT}}(\mu, \nu) =\min_{\boldsymbol{T} \in \Pi(\boldsymbol{\mu}, \boldsymbol{\nu})} \langle \boldsymbol{C}, \boldsymbol{T} \rangle + \epsilon \langle \boldsymbol{T}, \log \boldsymbol{T} \rangle
\end{equation}
%\vspace{-0.15cm}
where \( \epsilon > 0 \) controls the strength of regularization. The added entropy term \( \langle \boldsymbol{T}, \log \boldsymbol{T} \rangle \) promotes smoother transport plans and allows for efficient optimization via the Sinkhorn algorithm~\citep{distances2013lightspeed}. The optimization process can be completed in a few iterations, with the solution \( T^* \) being computed as:
\begin{equation}
T^* = \text{diag}(\mu^{(t)}) \exp(-\boldsymbol{C}/\epsilon) \text{diag}(\nu^{(t)}),
\end{equation}
where $t$ denotes the iteration number and in each iteration, the marginal distributions \(\mu^{(t)}=\mu / \left( \exp(-\boldsymbol{C}/\epsilon) \nu^{(t-1)} \right)\) \text{and} \(\nu^{(t)} = \nu / \left( \exp(-\boldsymbol{C}/\epsilon) \mu^{(t)} \right)\).

\paragraph{Fast Implementation of Dykstra’s Algorithm}
To efficiently solve the entropically regularized UOT problem defined in Eq.~\ref{eq:UOT}, we adopt a fast matrix-scaling variant of Dykstra’s algorithm. The full procedure is detailed in Algorithm~\ref{alg:dykstra}.

\paragraph{Generalized Cross-Entropy Loss}
To support the training objectives described in Eq.~(26)--(27), we provide a detailed explanation of the Generalized Cross-Entropy (GCE) loss~\citep{zhang2018generalized}, denoted as $\mathcal{L}_{\mathrm{gce}}$. This loss serves as the primary supervision signal for training, especially in the presence of label noise.

\label{A1}
\begin{algorithm}[t]
\caption{The training process of NA-MVP}
\textbf{Input:} Noisy dataset $\mathcal{D}_{\text{noisy}}$, pretrained CLIP model $f$, text encoder $\psi(\cdot)$, number of prompts $N$, entropy parameter $\epsilon$, total training epochs $T$, number of supervised epochs $T_{\text{sup}}$\par
\textbf{Output:} Optimized prompt parameter set $\Omega = \left\{ \omega^{c}_{m},\omega^{n}_{m} \right\}_{m=1}^{N}$
\label{alg:NA-MVP}
\begin{algorithmic}[1]
\For{$t = 1, 2, \dots, T$}
    \For{each mini-batch $\mathcal{B}_t$}
        \If{$t > T_{\text{sup}}$}
            \State Identify noisy samples using threshold \par \quad \quad \quad $\phi(p^n, p^c)$ and construct $\mathcal{D}_{\text{denoised}}$
        \EndIf
        \State Extract local feature map $F_i$ using $f$
        \State Generate prompt feature sets $G^c_k\in \mathbb{R}^{N \times d}$ and \par \quad \quad $G^n_k\in \mathbb{R}^{N \times d}$ for each class $k$
        \State Compute cost matrices $C^c_k = 1 - F_i G^c_k{}^\top$, \par \quad \quad $C^n_k = 1 - F_i G^n_k{}^\top$ using cosine similarity
        \State Solve UOT using Dykstra's algorithm:\par
        $
        \quad \quad T_k^{c*} = \text{diag}(\mu^{(t)}) \exp(-C^c_k / \epsilon) \text{diag}(\nu^{(t)}) $,\par
        $
        \quad \quad T_k^{n*} = \text{diag}(\mu^{(t)}) \exp(-C^n_k / \epsilon) \text{diag}(\nu^{(t)})
        $
        \State Compute UOT-based distances:\par
        \quad \quad $d^c_{\text{UOT}}(k) = \langle C^c_k, T_k^{c*} \rangle,  d^n_{\text{UOT}}(k) = \langle C^n_k, T_k^{n*} \rangle$
        \State Compute final prediction probabilities:\par
        \quad \quad $p(y = k \mid x_i) = (1 - p^n_{i,k}) \cdot p^c_{i,k}$
        \If{$t > T_{\text{sup}}$}
            \State Compute $\mathcal{L} = \mathcal{L}_{\text{gce}}$ using $\mathcal{D}_{\text{denoised}}$
        \Else
            \State Compute $\mathcal{L} = \mathcal{L}_{\text{gce}} + \lambda_i \cdot \mathcal{L}_{\text{itbp}}$ using $\mathcal{D}_{\text{noisy}}$
        \EndIf
        \State Update prompt parameters $\Omega$ with loss $\mathcal{L}$
    \EndFor
\EndFor
\State \Return $\Omega$
\end{algorithmic}
\end{algorithm}

% \begin{algorithm}[t]
% \caption{Fast Implementation of Dykstra’s Algorithm}
% \label{alg:dykstra}
% \textbf{Input:} Cost matrix $C$, marginal vectors $\mu$, $\nu$, entropic regularization parameter $\epsilon$
% \begin{algorithmic}[1]
% \State \textbf{Initialize:} $Q \gets \exp(-C/\epsilon),\ \nu^{(0)} \gets \mathds{1}_\nu,\ \Delta_\nu \gets \infty,\ \epsilon \gets 10^{-3}$
% \State Compute: 
% $Q_\mu \gets \dfrac{Q}{\mathrm{diag}(\mu)\mathds{1}_{|\mu| \times |\nu|}}$,\par$\quad Q_\nu^\top \gets \dfrac{Q^\top}{\mathrm{diag}(\nu)\mathds{1}_{|\mu| \times |\nu|}}$

% \For{$n = 1, 2, \dots$}{
%     \State $\mu^{(n)} \gets \min\left( \dfrac{\mathds{1}_{|\mu|}}{Q_\mu \nu^{(n-1)}},\ \mathds{1}_{|\mu|} \right)$
%     \State $\nu^{(n)} \gets \dfrac{\mathds{1}_{|\nu|}}{Q_\nu^\top \mu^{(n)}}$
%     \State $\Delta_\nu \gets \left\| \nu^{(n)} - \nu^{(n-1)} \right\|$
%     \If{$\Delta_\nu < \epsilon$}
%         \State \textbf{break}
%     \EndIf}
% \EndFor
% \State \Return $T^* = \mathrm{diag}(\mu^{(n)}) Q\ \mathrm{diag}(\nu^{(n)})$
% \end{algorithmic}
% \end{algorithm}

\begin{algorithm}[t]
\caption{Fast Implementation of Dykstra’s Algorithm}
\label{alg:dykstra}
\textbf{Input:} Cost matrix $C$, marginal vectors $\mu$, $\nu$, entropic regularization parameter $\epsilon$
\begin{algorithmic}[1]
\State \textbf{Initialize:} $Q \gets \exp(-C/\epsilon),\ \nu^{(0)} \gets \mathds{1}_\nu,\ \Delta_\nu \gets \infty,\ \epsilon \gets 10^{-3}$
\State Compute: \par
$Q_\mu \gets \dfrac{Q}{\mathrm{diag}(\mu)\mathds{1}_{|\mu| \times |\nu|}}, Q_\nu^\top \gets \dfrac{Q^\top}{\mathrm{diag}(\nu)\mathds{1}_{|\mu| \times |\nu|}}$
\For{$n = 1, 2, \dots$}
\State $\mu^{(n)} \gets \min\left( \dfrac{\mathds{1}_{|\mu|}}{Q_\mu \nu^{(n-1)}},\mathds{1}_{|\mu|} \right)$
\State $\nu^{(n)} \gets \dfrac{\mathds{1}_{|\nu|}}{Q_\nu^\top \mu^{(n)}}$
\State $\Delta_\nu \gets \left\| \nu^{(n)} - \nu^{(n-1)} \right\|$
\If{$\Delta_\nu < \epsilon$}
\State \textbf{break}
\EndIf
\EndFor
\end{algorithmic}
\end{algorithm}

The GCE loss is a noise-robust surrogate to the standard cross-entropy (CE) and mean absolute error (MAE) losses. Given a training sample $(x, y)$ where $y \in \{1, 2, \dots, C\}$ is the ground-truth label and $p = f(x) \in \Delta^{C-1}$ is the softmax output over $C$ classes, the GCE loss is defined as:
\begin{equation}
\mathcal{L}_{\mathrm{gce}}(x, y) = \frac{1 - p_y^q}{q}, \qquad 0 < q \leq 1,
\label{eq:gce}
\end{equation}
where $p_y$ denotes the predicted probability for class $y$, and $q$ is a tunable hyper-parameter that governs the degree of robustness. Following prior works, we fix $q = 0.5$ throughout all experiments, which offers a good trade-off between noise robustness and optimization stability.

\paragraph{Image-Text Bi-directional Prompt Loss}
Drawing inspiration from the bi-directional contrastive loss in CLIPN~\citep{wang2023clipn}, 
we introduce an auxiliary loss termed ITBP within our framework. 
This loss ensures image features remain close to semantically consistent prompts while avoiding confusion with incorrect or unrelated noisy prompts. 

Specifically, we distinguish between two types of matches: 
(1) \textbf{reversed match}, where the image matches its own noisy prompt that expresses opposite semantics, and 
(2) \textbf{unrelated match}, where the image is compared with other noisy prompts that are semantically irrelevant but not intentionally contradictory.
To encode this relationship, we define a binary match indicator \( m(x_i, t_j^{\text{n}}) \) between the \( i \)-th image and the \( j \)-th noisy prompt as:
%\vspace{-0.15cm}
\begin{equation}
m(x_i, t_j^{\text{n}}) = m_{ij} =
\begin{cases}
0, &i = j, \text{(reversed match)} \\
1, &i \neq j, \text{(unrelated match)}
\end{cases}
\end{equation}
The matched probability between image \( x_i \) and the \( j \)-th noisy prompt \( t_j^{\text{n}} \) is computed as:
\begin{equation}
p_{ij}^{\text{n}} = \frac{\exp(s_{i,j}^n / \tau)}{\exp(s_{i,j}^c/ \tau) + \exp(s_{i,j}^n / \tau)}
\end{equation}
The ITBP loss is formulated as:
\begin{equation}
\begin{split}
\mathcal{L}_{\text{itbp}} =-\frac{1}{N} \sum_{i=1}^{N} (1 - m_{ii}) \log(1 - p_{ii}^{\text{n}}) - \\ \frac{1}{N(N-1)} \sum_{i=1}^{N} \sum_{j \neq i} m_{ij} \log(p_{ij}^{\text{n}})
 \end{split}
\end{equation}%\vspace{-0.25cm}

\section{Experimental Details}
\subsection{Dataset Details}
\label{dataset}
We selected six representative visual classification datasets as benchmarks. The detailed statistics of each dataset are shown  in Table \ref{tab:1}, including the original task, the number of classes, and the sizes of training and test samples.

\begin{table*}[ht]
\centering
\caption{The detailed statistics of datasets used in experiments.}
\label{tab:1}
\setlength{\tabcolsep}{10pt}
\begin{tabular}{l l c r r}
\toprule
\textbf{Dataset} & \textbf{Task} & \textbf{Classes} & \textbf{Training Size} & \textbf{Testing Size} \\
\midrule
Caltech101~\citep{fei2004learning}     & Object recognition              & 100 & 4,128   & 2,465  \\
DTD~\citep{cimpoi2014describing}            & Texture recognition              & 47  & 2,820   & 1,692  \\
Flowers102~\citep{nilsback2008automated}     & Fine-grained flowers recognition & 102 & 4,093   & 2,463  \\
OxfordPets~\citep{parkhi2012cats}     & Fine-grained pets recognition    & 37  & 2,944   & 3,669  \\
UCF101~\citep{peng2018two}         & Video action recognition         & 101 & 7,639   & 3,783  \\
Food101N~\citep{lee2018cleannet} & Fine-grained food recognition    & 101 & 310,009 & 30,300 \\
\bottomrule
\end{tabular}
\end{table*}
\subsection{Implementation details}
\label{B2}
All input images are resized to \(224 \times 224\) and divided into \(14 \times 14\) patches of dimension 768. For the Unbalanced OT problem in Eq.~\ref{eq:6}, we set the entropic regularization weight to \(\epsilon = 0.1\) and the marginal relaxation parameter to \(\theta = 0.9\). The loss balancing coefficient \(\lambda_{\text{i}}\) is set to 0.1. The maximum number of iterations in Algorithm~\ref{alg:dykstra} is set to 100, with early stopping applied when \(\Delta_\nu < 0.01\).
We use 16 shared context tokens appended to the class token, each of dimension 512. Prompts are randomly initialized and inserted at the "end" token position.
Batch sizes are set to 32 for training and 100 for
testing. The total number of training epochs is 50, with 20 for the supervised phase and 30 for semi-supervised refinement. Warm-up is set to 1 epoch for all datasets, except for the Flowers dataset, which adopts a 20-epoch warm-up. All experiments are conducted on a single NVIDIA GeForce RTX 4090 GPU.
\subsection{Noisy label identification motivation}
\label{moti}
To validate the intuition behind our noisy label identification strategy, we conduct a case study on the Caltech101 dataset. Samples are grouped into clean and noisy subsets based on their ground-truth annotations. We visualize the epoch-wise average values of the clean prompt confidence \( p^c \) and the adaptive threshold \( \phi \) for both groups. 

As shown in Figure~\ref{fig:motivation}, clean samples exhibit consistently high values of \( p^c \), while their corresponding \( \phi \) remains close to zero. In contrast, noisy samples demonstrate the opposite pattern: \( \phi \) is significantly larger than \( p^c \), especially in the early training phase. %This clear contrast empirically supports the effectiveness of our threshold-based criterion defined in Eq.~(18).
These trends confirm that our bi-directional alignment framework provides a meaningful signal to distinguish between clean and noisy labels. Moreover, the observed dynamics further justify the design of our selective noisy label refinement strategy introduced in Section~\ref{4.1}, which integrates soft thresholding with OT-based pseudo-label correction.

\begin{figure}[t]
    \centering
    % \setlength{\abovecaptionskip}{0.cm}
    % \setlength{\belowcaptionskip}{-0.cm}
    % 子图1
    \begin{subfigure}{0.35\linewidth}
        % \centering  
        \includegraphics[width=1.25\textwidth]{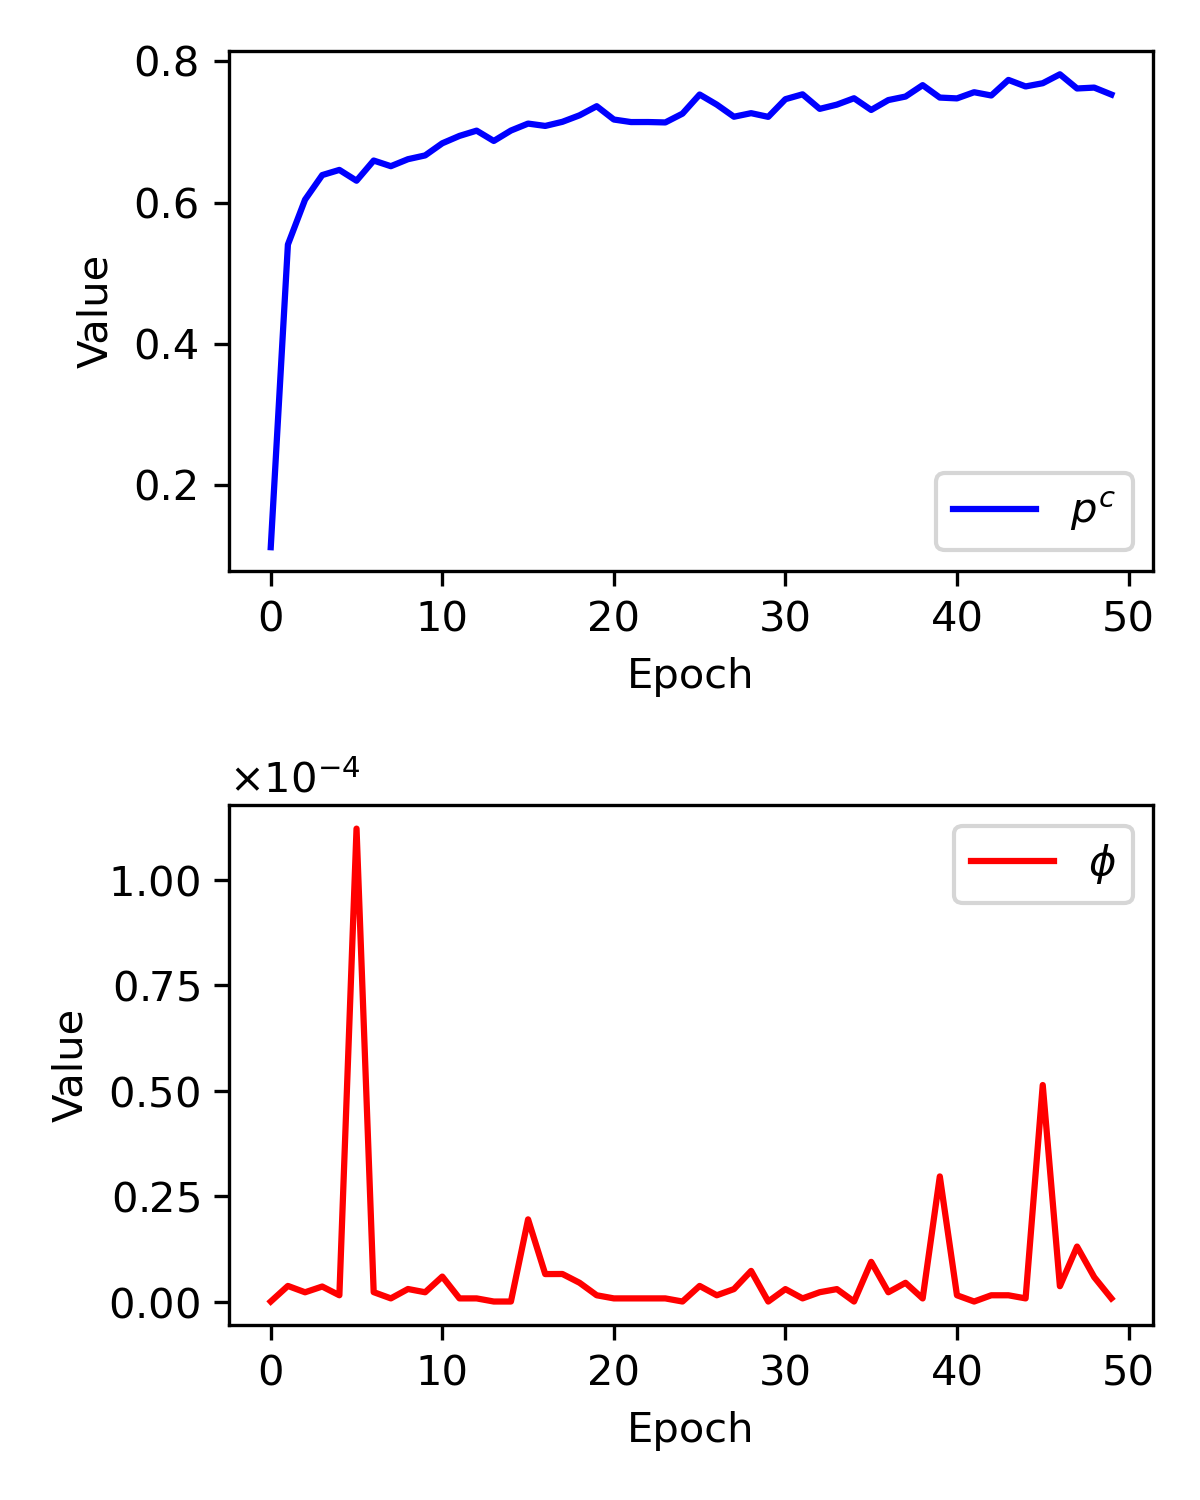}
        \caption{Clean samples}
    \end{subfigure}\hspace{10mm}
    % 子图2
    \begin{subfigure}{0.35\linewidth}
        \centering  
        \includegraphics[width=1.25\textwidth]{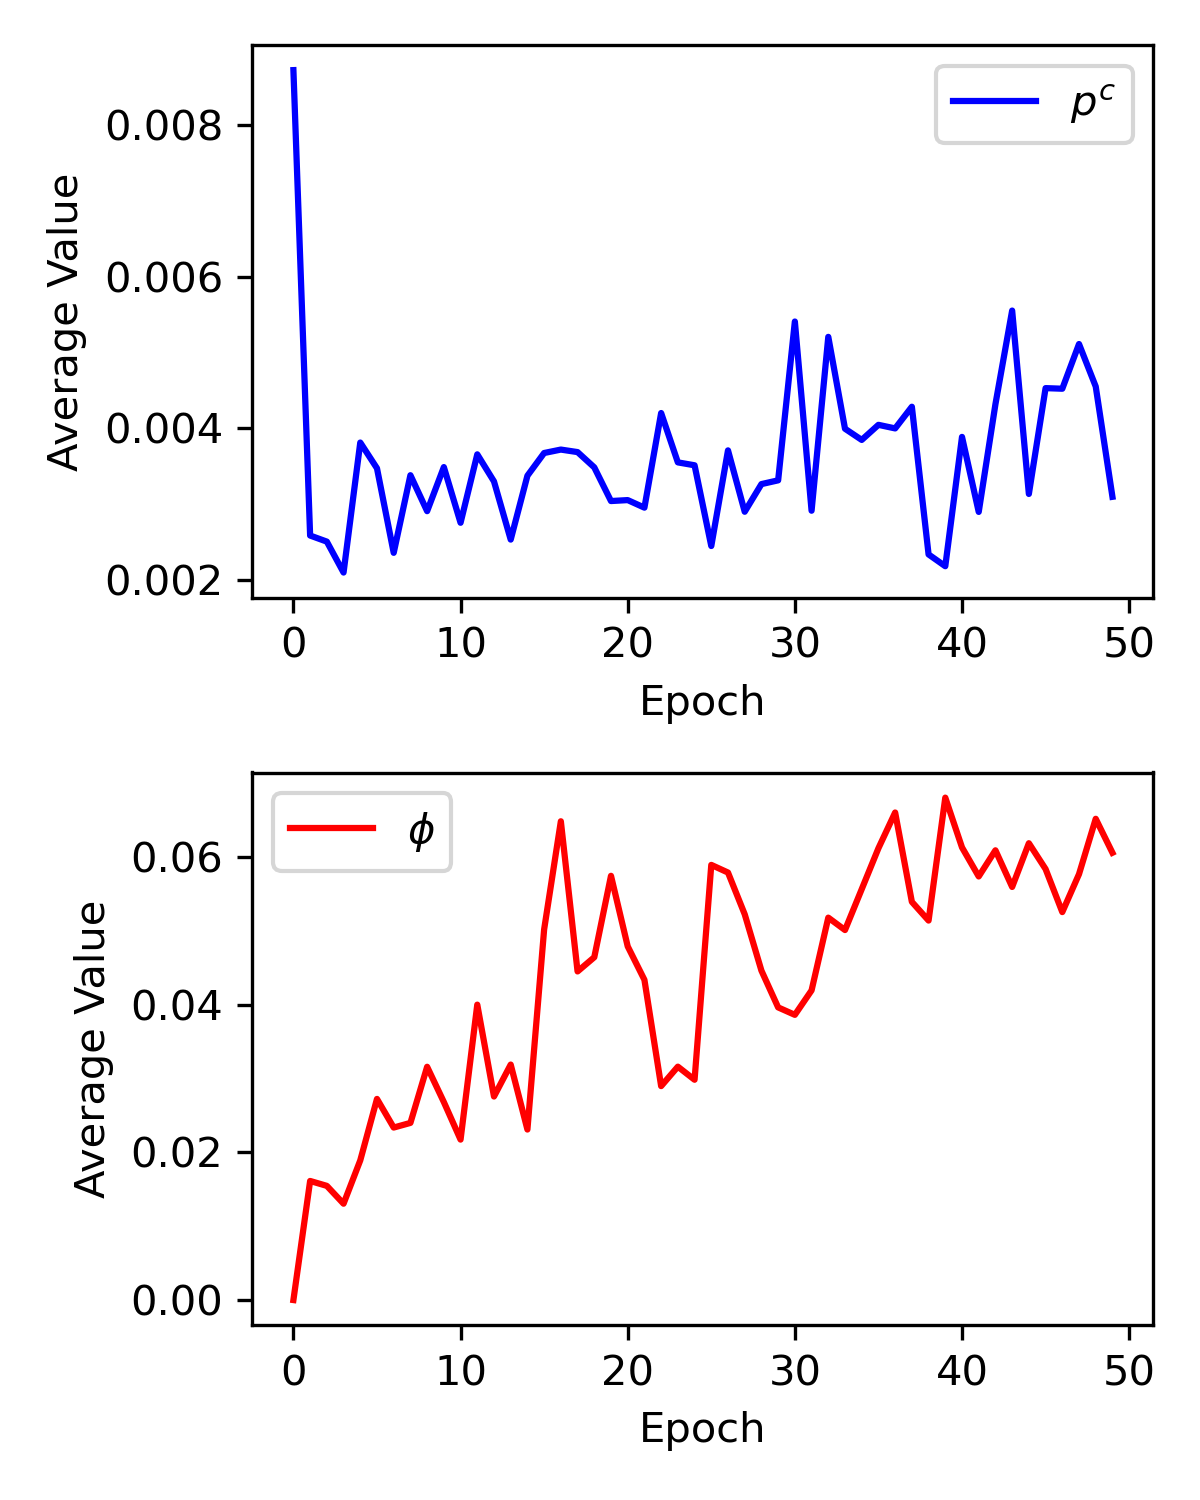}
        \caption{Noisy samples}
    \end{subfigure}
    \caption{Behavioral differences of $p^c$ and $\phi$ on clean vs. noisy samples in Caltech101. 
    }
    \label{fig:motivation}
\end{figure}

\section{Additional Experimental results}
%\vspace{-7pt}
\subsection{Effect of Selective Refinement with $\phi_{i,k}$}
\label{refinement}

\begin{figure*}[t]
    \centering
    % 子图1
    \begin{subfigure}{0.325\linewidth}
        \centering  
        \includegraphics[width=0.950\textwidth]{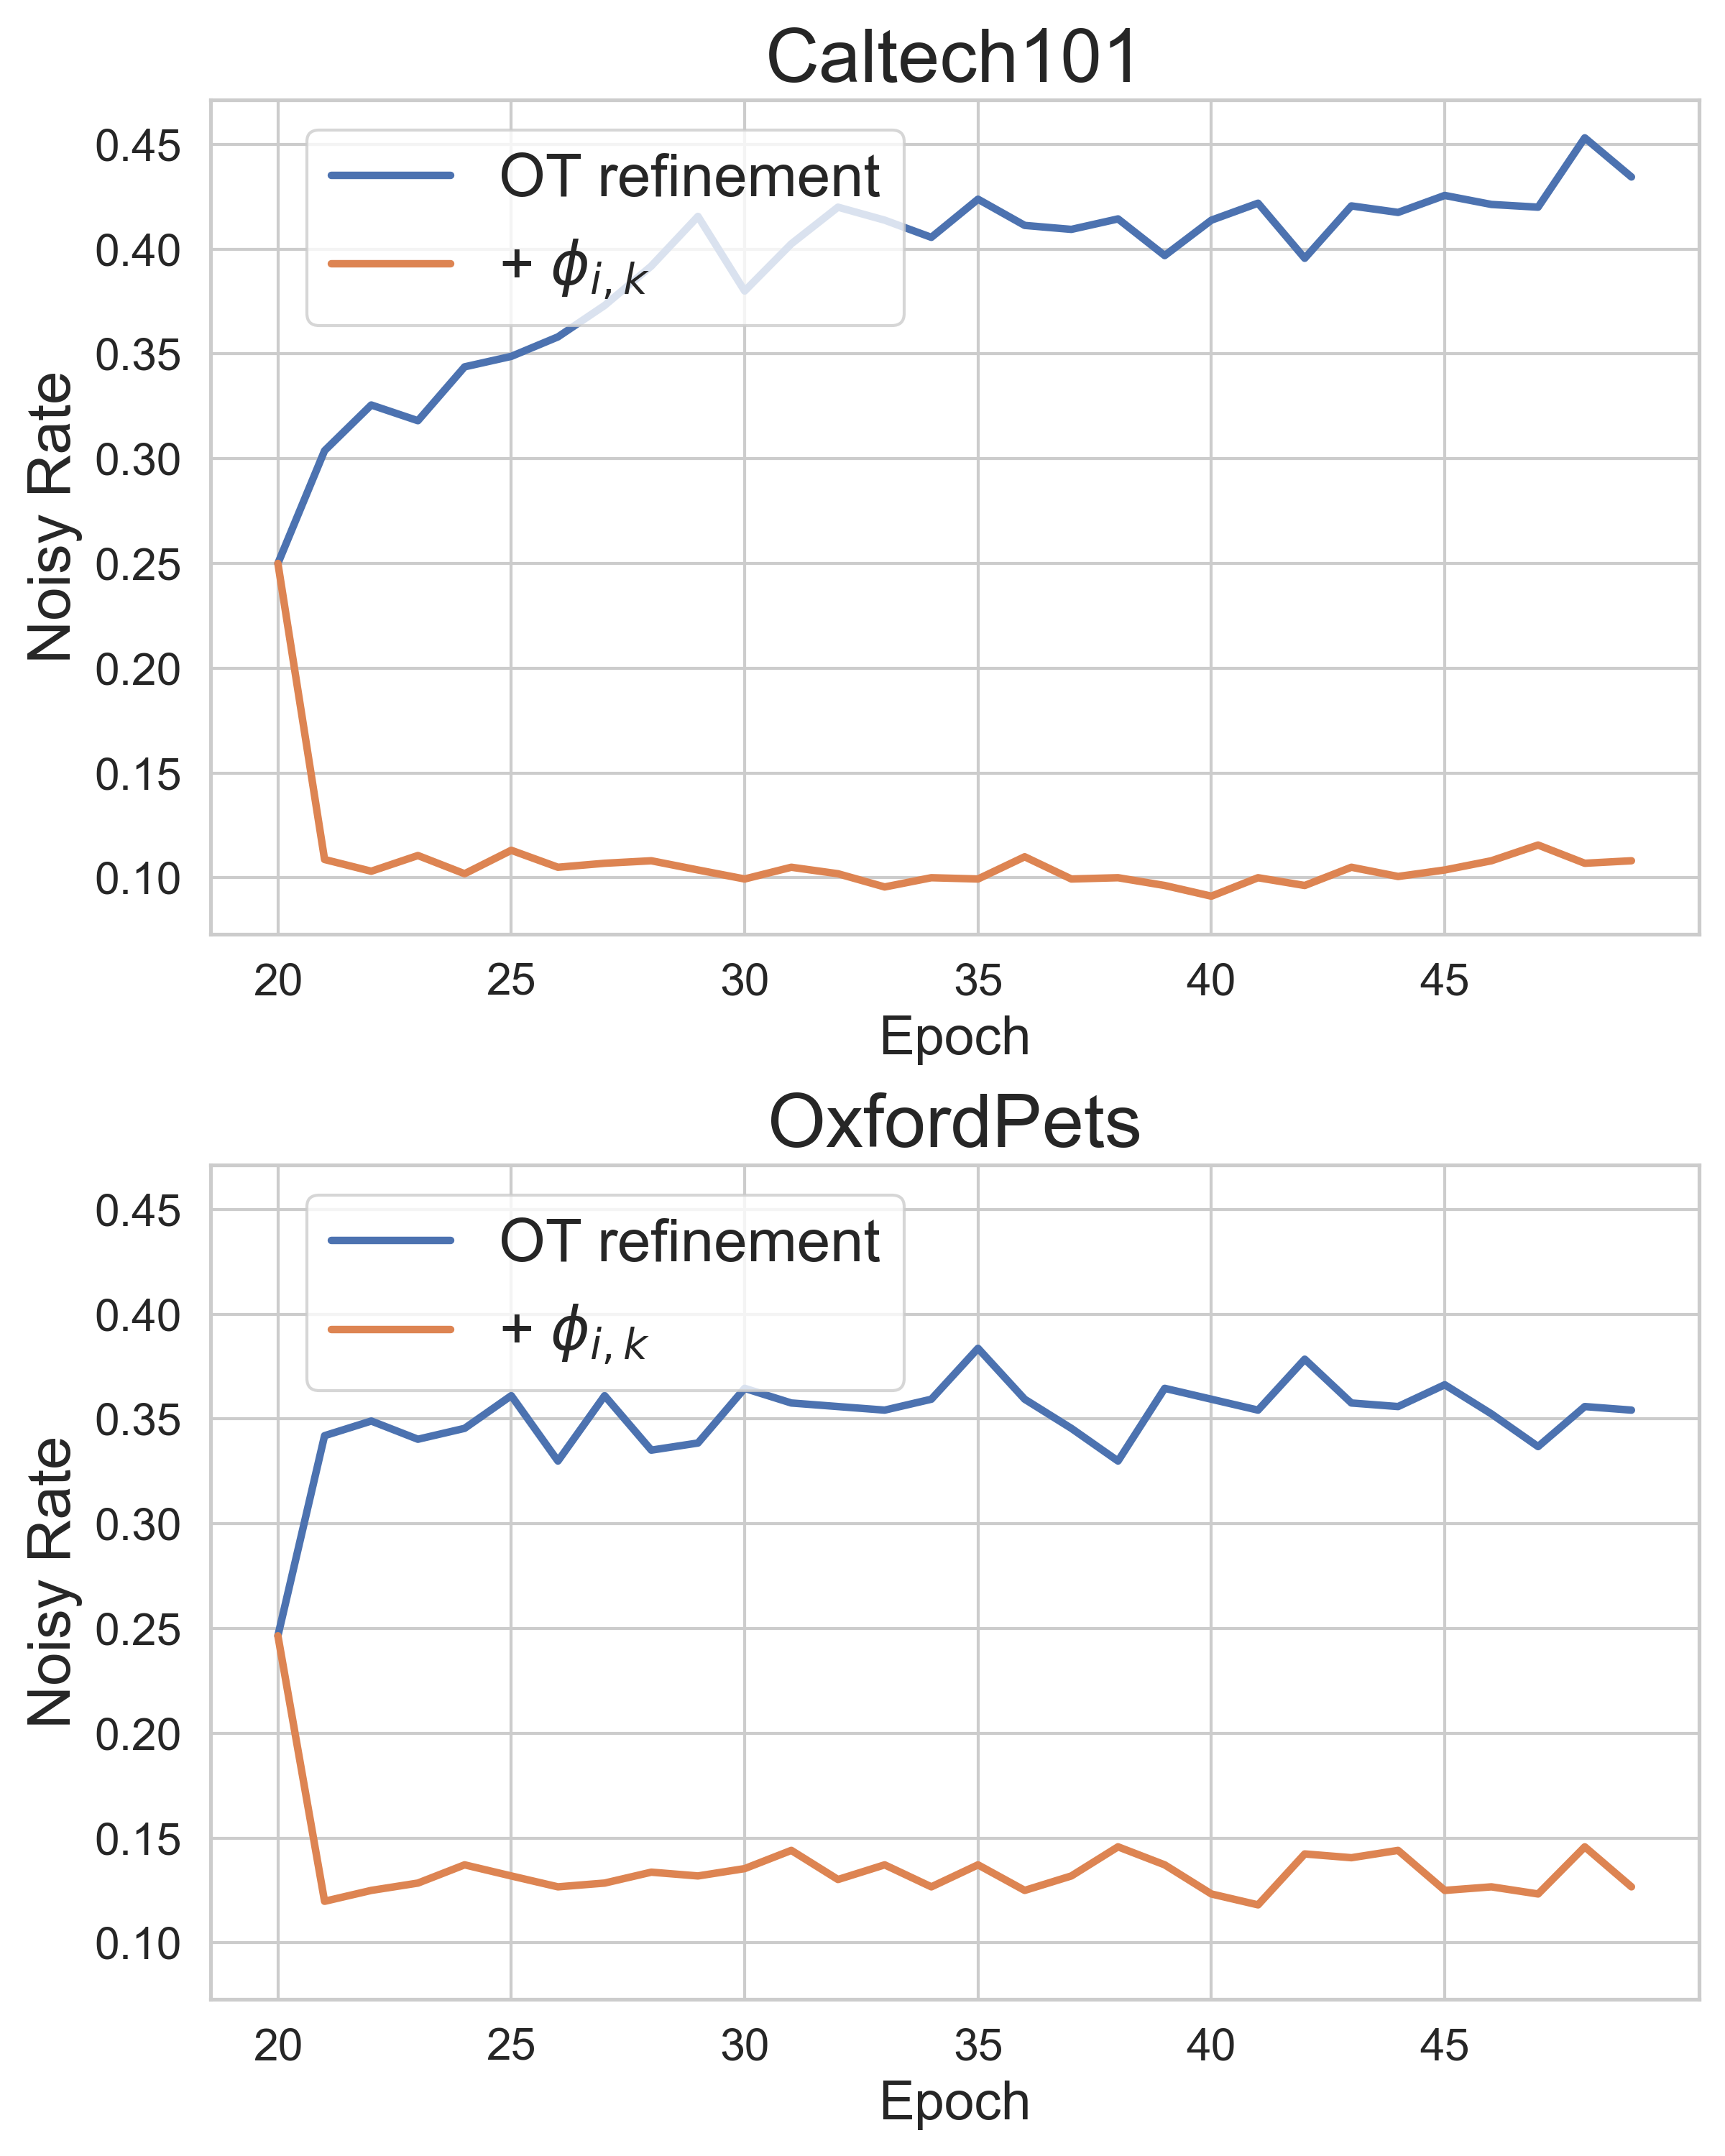}
        \caption{Noise rate = 25\%}
    \end{subfigure}
    % 子图2
    \begin{subfigure}{0.325\linewidth}
        \centering
        \includegraphics[width=0.950\textwidth]{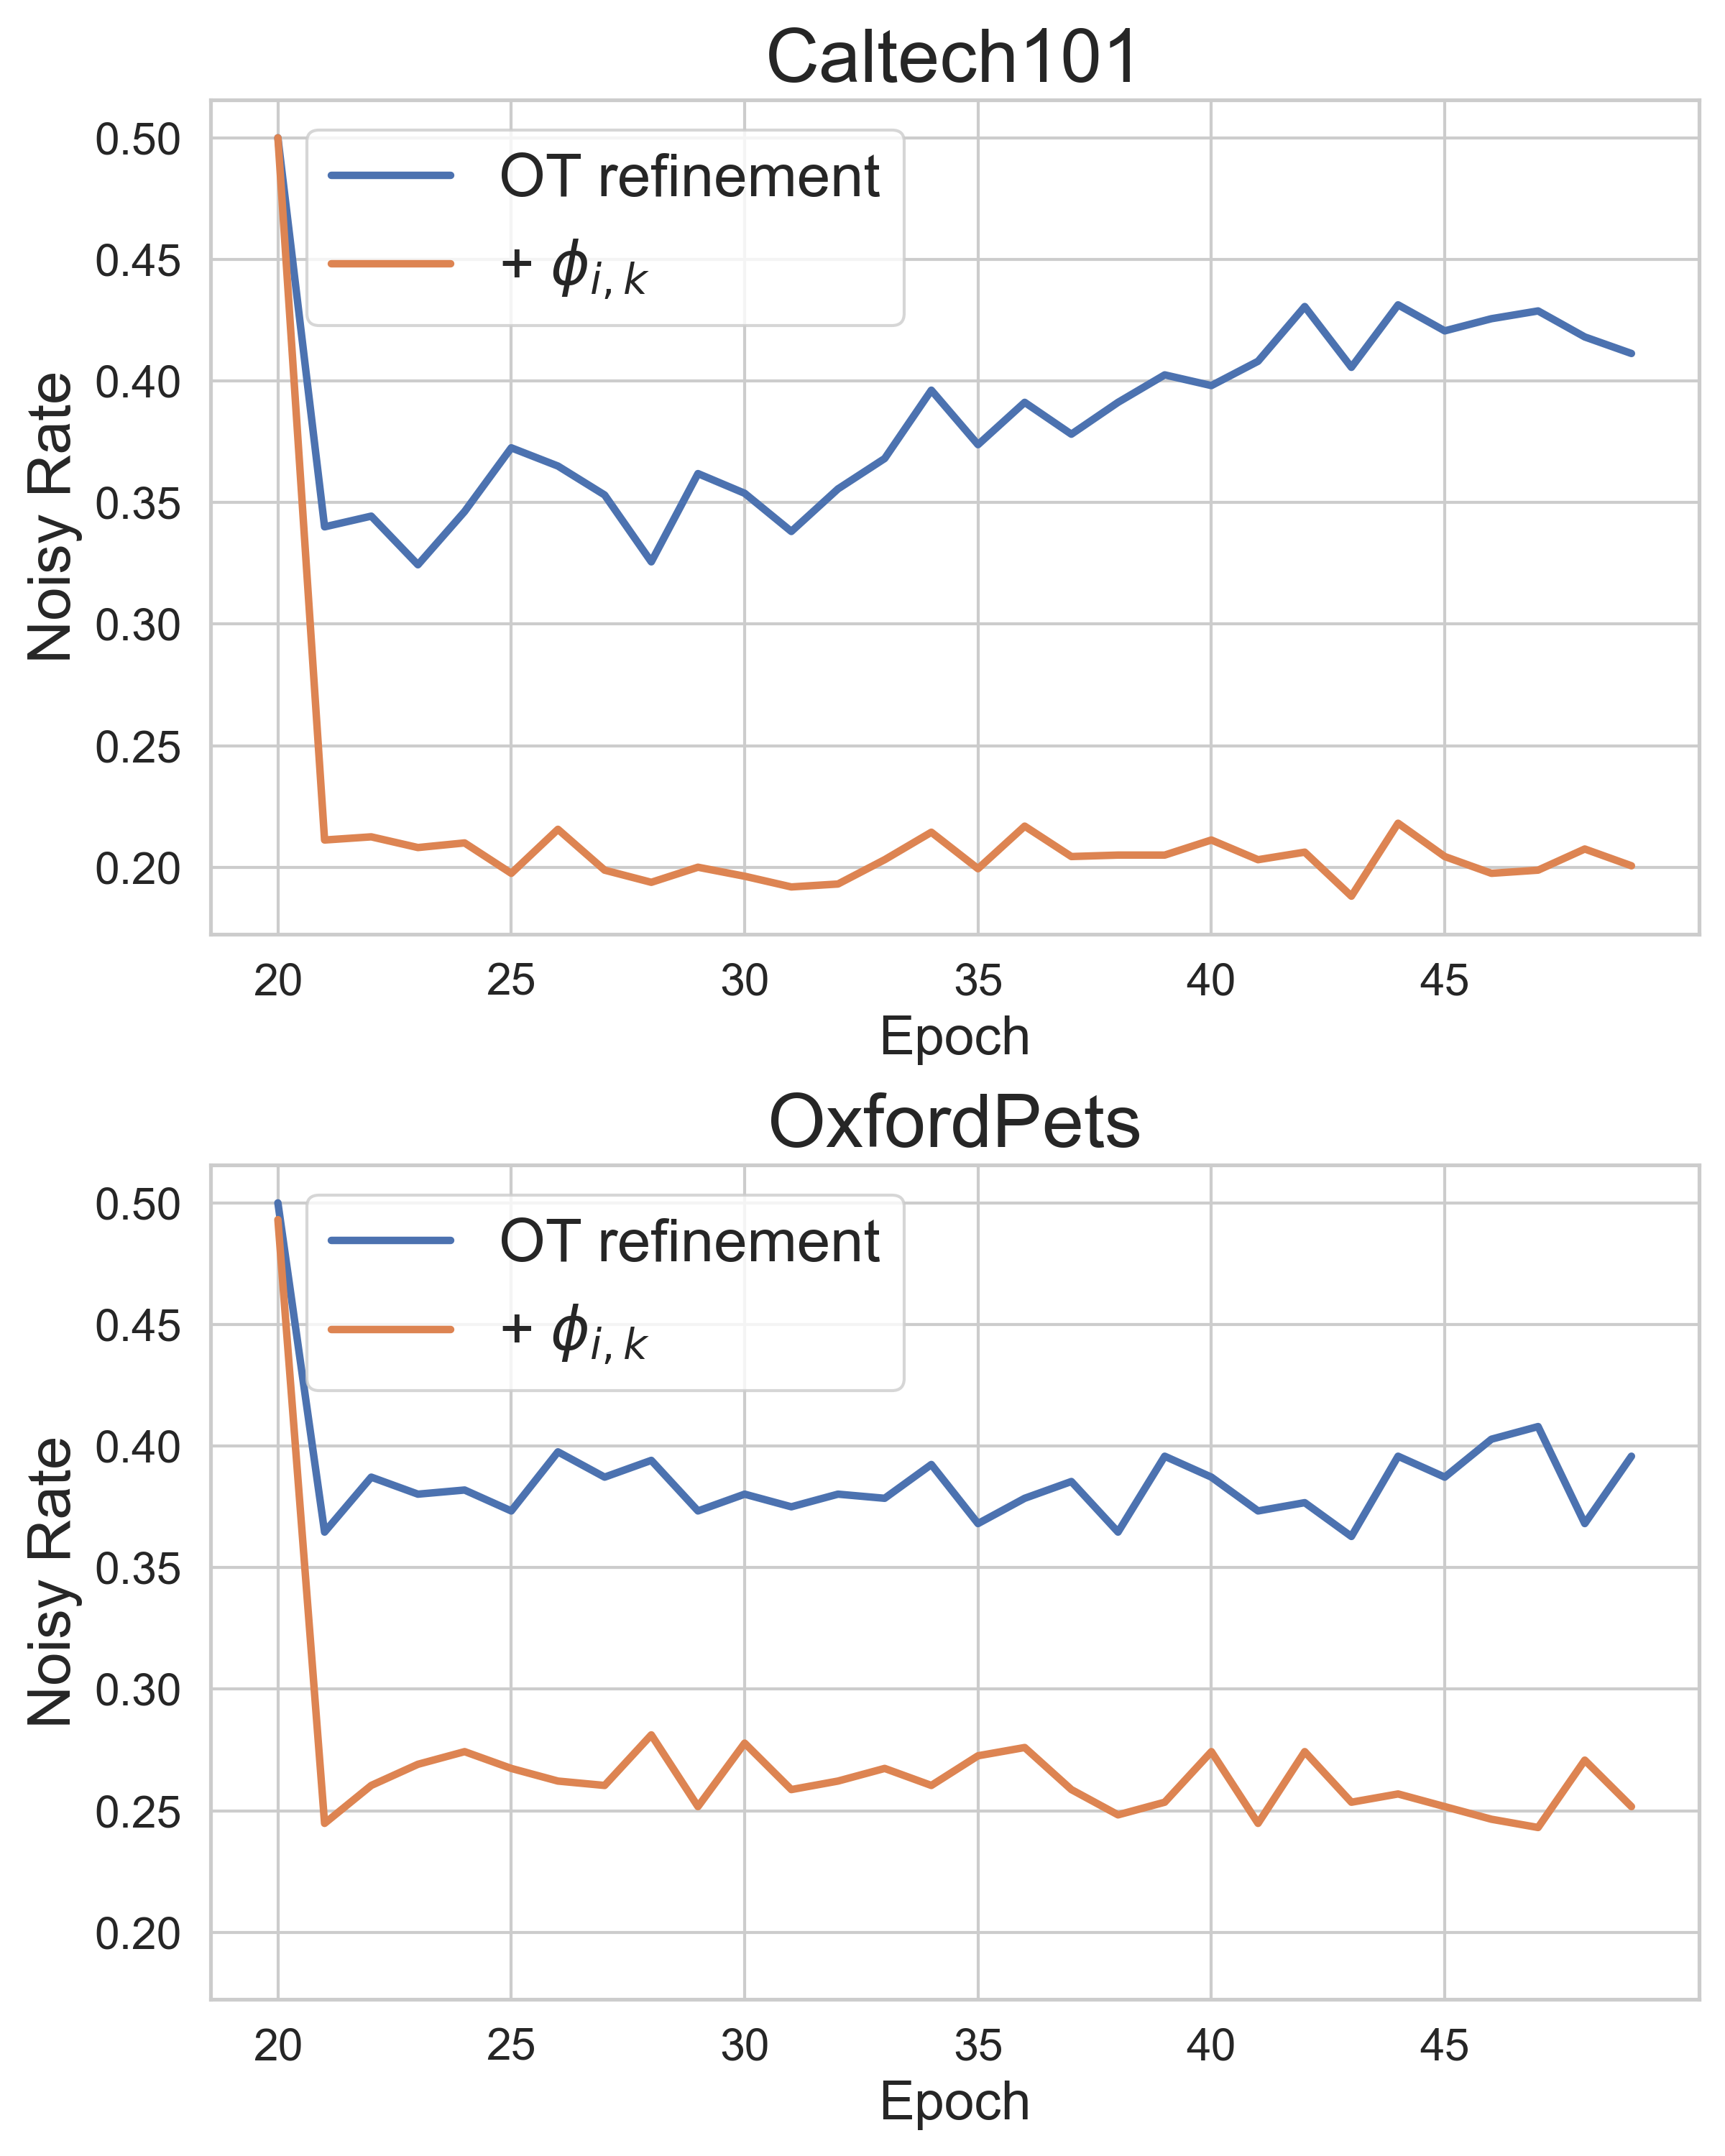}
        \caption{Noise rate = 50\%}
        
    \end{subfigure}
    % 子图3
    \begin{subfigure}{0.325\linewidth}
        \centering
        \includegraphics[width=0.950\textwidth]{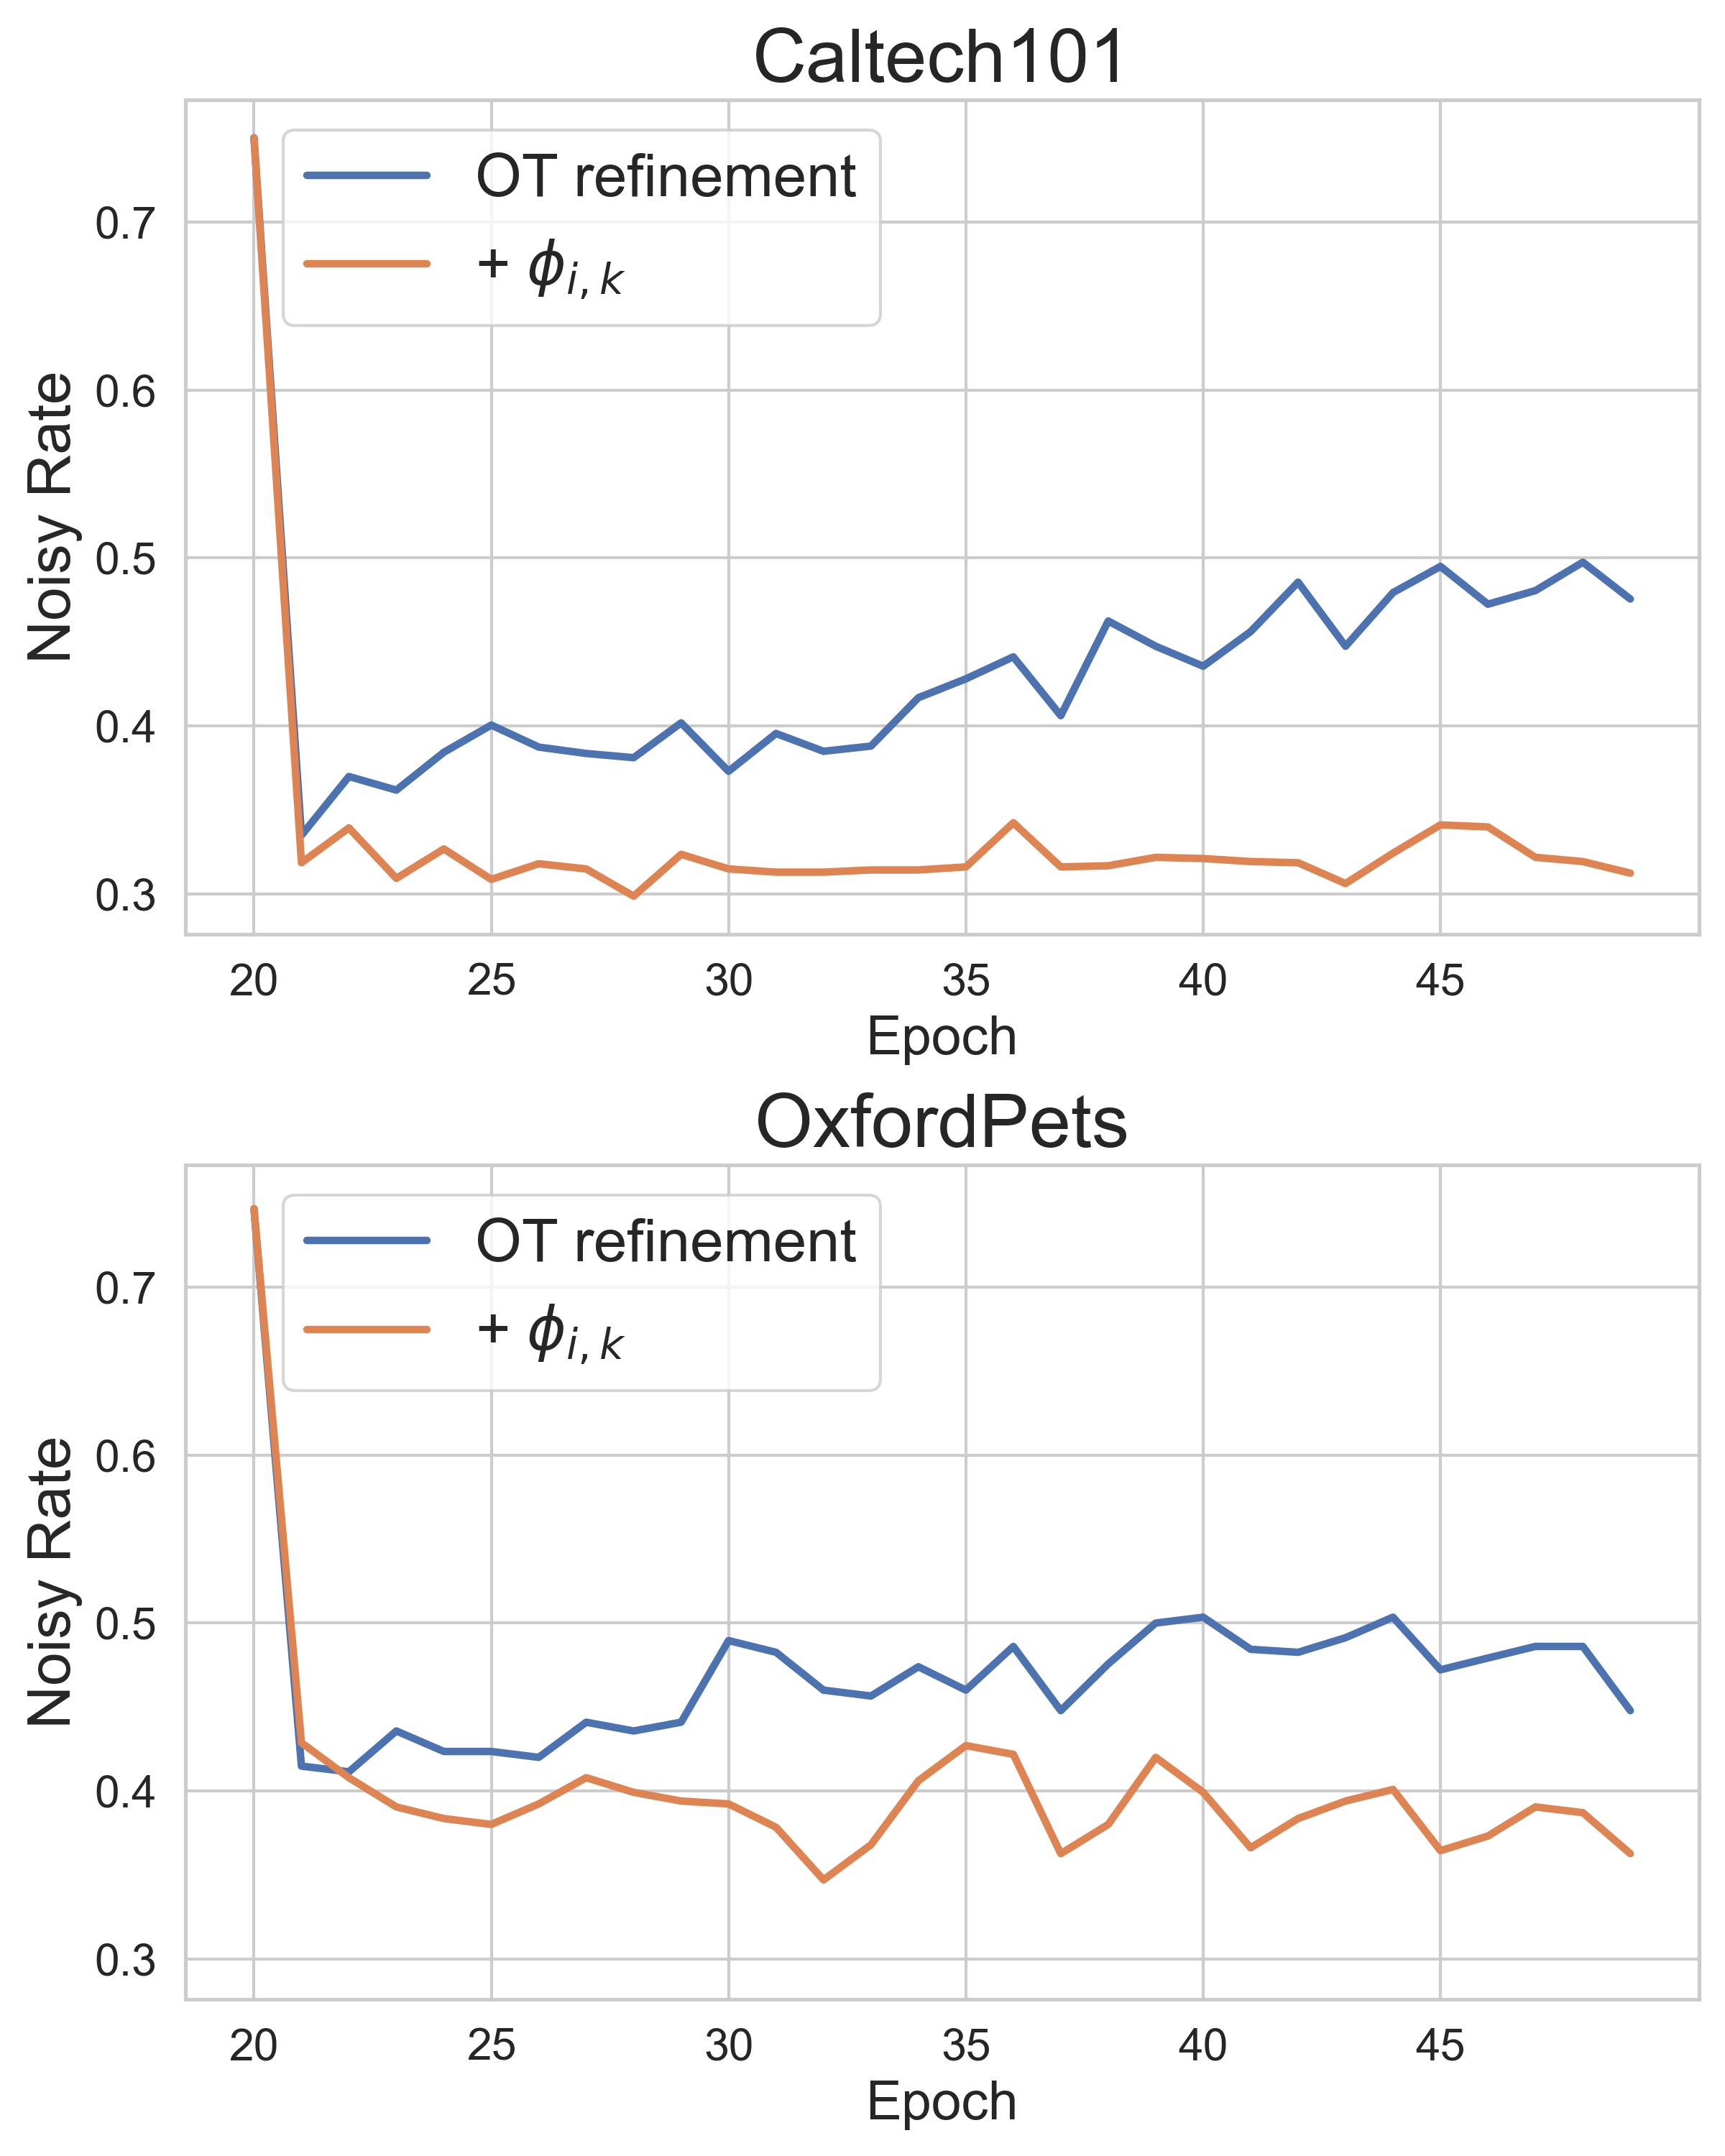}
        \caption{Noise rate = 75\%}
        
    \end{subfigure}
    \caption{Comparison of  OT refinement and selective refinement with $\phi_{i,k}$ under different noise rates on Caltech101 and OxfordPets datasets.
    }
    \label{OT refine}
    % \vspace{-10pt}
\end{figure*}

% \begin{table}[t]
% \centering
% \setlength{\tabcolsep}{2.5pt}
% \renewcommand{\arraystretch}{1}
% \caption{The accuracy comparison on OxfordPets Dataset. }
% \label{tab:DEFT}
% \begin{tabular}{lcccccc}
% \toprule
% Noise rate & 12.5\% & 25\% & 37.5\% & 50\% & 62.5\% & 75\%  \\
% \midrule
% DEFT~\citep{wei2024vision}& \textbf{88.83} & 88.23 & 88.10 & 86.73 & 84.10 & 75.87 \\
% NA-MVP            & 88.50 & \textbf{88.40} & \textbf{88.23} & \textbf{88.13} & \textbf{86.93} & \textbf{86.23} \\
% \bottomrule
% \end{tabular}
% \end{table}
To further analyze the effectiveness of our proposed selective label refinement guided by $\phi_{i,k}$, we compare the evolution of noisy label ratio over training epochs under different settings. As shown in Figure \ref{OT refine}, we visualize the noisy rate curves during training on Caltech101 and OxfordPets under three synthetic noise levels: 25\%, 50\%, and 75\%. We compare the baseline OT refinement strategy with our selective refinement method guided by $\phi_{i,k}$. Across all datasets and noise settings, we observe that the noisy rate decreases more significantly and remains consistently lower when using $\phi_{i,k}$-guided refinement. This indicates that our method effectively filters out potentially clean samples from aggressive relabeling, preventing overcorrection and improving the quality of pseudo-labels. 

We further quantify the effectiveness of our selective refinement by evaluating the corresponding correction accuracy. For example, on Caltech101, our method reduces the noise ratio from 0.50 to 0.19, achieving a correct correction rate of 73.7\%; under 0.75 noise, it decreases to 0.31 with a 71.4\% correct rate. These findings further demonstrate that $\phi_{i,k}$ improves label correction reliability by enabling a more conservative and noise-aware refinement process. 
\begin{table*}[t]
\centering
\setlength{\tabcolsep}{10pt}
\caption{The accuracy comparison across datasets and noise levels. (\%)}
\label{tab:plot}
% \resizebox{\textwidth}{!}{ % Automatically scale the table to fit the page
\begin{tabular}{
  >{\centering\arraybackslash}m{1.5cm} %
  >{\centering\arraybackslash}m{1.5cm} %Dataset
  *{6}{c}                               % Symmetric noise levels
  *{2}{c}                               % Asymmetric noise levels
}
\toprule
\multirow{2}{*}{Dataset} & \multirow{2}{*}{Method} 
& \multicolumn{6}{c}{Noise rate: Sym} 
& \multicolumn{2}{c}{Noise rate: Asym} \\
& & 0.125 & 0.25 & 0.375 & 0.5 & 0.625 & 0.75 & 0.25 & 0.5 \\
\midrule
\multirow{2}{*}{Caltech101}
& PLOT~\citep{chen2022plot} & 90.03 & 88.10 & 85.13 & 84.10 & 75.90 & 62.70 & 81.17 & 50.80 \\
& NA-MVP & \textbf{92.07} & \textbf{92.10} & \textbf{91.60} & \textbf{91.30} & \textbf{90.07} & \textbf{89.37} & \textbf{91.47} & \textbf{89.53} \\
\midrule
\multirow{2}{*}{DTD}
& PLOT~\citep{chen2022plot} & 60.27 & 56.87 & 50.77 & 44.67 & 36.53 & 23.57 & 52.80 & 32.03 \\
& NA-MVP & \textbf{63.73} & \textbf{63.13} & \textbf{61.63} & \textbf{58.50} & \textbf{52.93} & \textbf{48.63} & \textbf{62.33} & \textbf{52.10} \\
\midrule
\multirow{2}{*}{Flowers102}
& PLOT~\citep{chen2022plot} & 91.63 & 89.00 & 84.67 & 77.10 & 66.80 & 47.57 & 76.20 & 40.60 \\
& NA-MVP & \textbf{94.20} & \textbf{93.30} & \textbf{92.00} & \textbf{90.47} & \textbf{85.07} & \textbf{76.47} & \textbf{91.37} & \textbf{78.43} \\
\midrule
\multirow{2}{*}{OxfordPets}
& PLOT~\citep{chen2022plot} & 84.57 & 79.43 & 74.70 & 64.60 & 52.10 & 41.50 & 73.87 & 44.47 \\
& NA-MVP & \textbf{88.50} & \textbf{88.40} & \textbf{88.23} & \textbf{88.13} & \textbf{86.93} & \textbf{86.23} & \textbf{87.53} & \textbf{79.33} \\
\midrule
\multirow{2}{*}{UCF101}
& PLOT~\citep{chen2022plot} & 73.30 & 69.37 & 65.27 & 59.13 & 51.50 & 40.93 & 61.33 & 36.43 \\
& NA-MVP & \textbf{75.33} & \textbf{74.03} & \textbf{72.30} & \textbf{70.93} & \textbf{68.43} & \textbf{63.93} & \textbf{73.40} & \textbf{65.40} \\
\bottomrule
\end{tabular}
% }
\end{table*}
% Additionally, we conducted further experiments on the OxfordPets dataset to compare our method with DEFT~\citep{wei2024vision}. DEFT selects clean samples using the rule: $p^{\text{clean}}_{ik} > 0.5$. The results, summarized in Table \ref{tab:DEFT}, show that NA-MVP consistently outperforms DEFT across all noise levels, particularly under higher noise ratios. These results reinforce the effectiveness of our method in handling noisy data, especially in scenarios with high noise levels, where our adaptive approach offers a significant improvement over the baseline methods.
\begin{table}[t]
\centering
\setlength{\tabcolsep}{2pt}

\caption{Performance comparison with unsupervised medthods.}
\label{tab:unsupervised}
\small
\begin{tabular}{lcccccc}
\toprule
Method & OxfordPets & DTD & UCF101 & Flowers102 \\
\midrule
MetaPrompt~\citep{mirza2024meta} & 88.10 & 50.80 & 67.90 & 73.90 \\
LaFTer~\citep{mirza2023lafter} & 82.70 & 46.10 & 68.20 & 71.00 \\
NA-MVP (25\% noise) & \textbf{88.40} & \textbf{63.10} & \textbf{74.00} & \textbf{93.30} \\
NA-MVP (50\% noise) & \textbf{88.13} & \textbf{58.50} & \textbf{70.93} & \textbf{90.47} \\
NA-MVP (75\% noise) & 86.23 & 48.63 & 63.93 & \textbf{76.47} \\
\bottomrule
\end{tabular}
\end{table}
\subsection{Analysis of the Number of Multi-view Prompts}
\label{imbalanced}
\begin{table}[t]
\centering
\caption{Experimental results under imbalanced numbers of prompts on DTD and OxfordPets.}
\small
\setlength{\tabcolsep}{1.8pt}
\begin{tabular}{lcccccccc}
\toprule
Datasets & \multicolumn{4}{c}{DTD} & \multicolumn{4}{c}{OxfordPets} \\
Noise rate & 0.25 & 0.5 & 0.75 & Avg. & 0.25 & 0.5 & 0.75 & Avg. \\
\midrule
N=1  & 62.36 & 57.33 & 47.24 & 55.64 & 88.27 & 87.23 & 85.26 & 86.92 \\
N=2  & 62.86 & 57.17 & 47.40 & 55.81 & 88.20 & 87.59 & 85.50 & 87.10 \\
N=4  & \textbf{63.13} & \textbf{58.50} & \textbf{48.63} & \textbf{56.75} & 88.40 & \textbf{88.13} & \textbf{86.23} & \textbf{87.59} \\
N=8  & 62.76 & 57.07 & 47.37 &55.73 & \textbf{88.57} & 87.63 & 85.73 & 87.31 \\
\bottomrule
\end{tabular}
\end{table}
To investigate the effect of imbalanced numbers of clean and noisy prompts, we conduct experiments by fixing the number of clean prompts to 4 while varying the number of noisy prompts (N = 1, 2, 4, 8). The evaluation is performed under different noise rates on the DTD and OxfordPets datasets. The results clearly show that the best performance is achieved when the number of noisy prompts equals the number of clean prompts (i.e., N=4). This trend is particularly evident under higher noise rates, indicating that a balanced prompt configuration enhances model robustness to noise.

\subsection{Comparison with other methods}
\label{other comparison}
\paragraph{Comparison with PLOT}
PLOT~\citep{chen2022plot} utilizes OT to align image and prompt features for few-shot classification and inspired us to identify noisy labels from multi-view. While PLOT has shown great promise, our method, NA-MVP, improves upon this by integrating multi-view prompt learning and a UOT-based denoising strategy, particularly effective in high-noise conditions. To validate NA-MVP, we compared it with PLOT under various noise levels. As shown in Table \ref{tab:plot}, NA-MVP consistently outperforms PLOT in all datasets and noise settings, with a particularly significant advantage under higher noise conditions. These results emphasize the robustness of our framework in handling noisy labels, supporting the effectiveness of our approach in noisy regimes.

\paragraph{Comparison with unsupervised methods}
Although few-shot learning generally outperforms unsupervised methods, we recognize the importance of empirically evaluating whether learning from noisy few-shot labels can yield meaningful improvements. In this regard, we compared NA-MVP with two recent unsupervised methods: MetaPrompt~\citep{mirza2024meta} and LaFTer~\citep{mirza2023lafter}. As shown in Table \ref{tab:unsupervised}, NA-MVP outperforms both MetaPrompt and LaFTer across most datasets. Even at higher noise levels (50\% and 75\%), our method remains competitive or superior. These results demonstrate that learning from a small amount of noisy supervision, when appropriately modeled, can be more effective than training with no labeled data. This underscores the practical value of noisy few-shot learning in real-world low-resource scenarios.

\paragraph{Comparison with NBNN}
We also compared NA-MVP with NBNN~\citep{boiman2008defense}, a widely used set-to-set matching method with cosine similarity as a distance metric. Our experiments on the Caltech101 and OxfordPets datasets show that NA-MVP consistently outperforms NBNN across different noise levels, particularly under higher noise conditions. The results in Table \ref{tab:nbnn} indicate that UOT-based matching in NA-MVP provides a more robust and adaptive alignment between prompts and image features, especially when class distributions are corrupted or ambiguous.

\begin{table*}[t]
\centering
\setlength{\tabcolsep}{8pt}

\caption{Impact of the loss balancing coefficient $\lambda_{\text{i}}$ under different noise rates. (\%)}
\begin{tabular}{lccccccccc}
\toprule
Datasets & \multicolumn{3}{c}{DTD} & \multicolumn{3}{c}{OxfordPets} & \multicolumn{3}{c}{UCF101} \\
Noise rate & 0.25 & 0.5 & 0.75& 0.25 & 0.5 & 0.75& 0.25 & 0.5 & 0.75 \\
\midrule
$\lambda_{\text{i}}$=0.01 & 62.36 & 57.96 & 48.09 & 88.37 & 87.93 & 85.43 & 73.53 & 70.57 & 61.87 \\
$\lambda_{\text{i}}$=0.05 & 62.03 & 58.10 & 48.39 & \textbf{88.53} & \textbf{88.37} & 85.90 & 73.60 & \textbf{71.09} & 62.90 \\
$\lambda_{\text{i}}$=0.1  & \textbf{63.13} & \textbf{58.50} & \textbf{48.63} & 88.40 & 88.13 & \textbf{86.23} & \textbf{74.03} & 70.93 & \textbf{63.93} \\
$\lambda_{\text{i}}$=0.5  & 62.96 & 57.33 & 47.19 & 88.33 & 87.50 & 85.33 & 73.63 & 69.13 & 60.74 \\
\bottomrule
\label{tab:lambda_study}
\end{tabular}
\end{table*}

\begin{table}[t]
\centering
\small
\setlength{\tabcolsep}{1.6pt}

\caption{Performance comparison on Caltech101 and OxfordPets. (\%)}
\label{tab:nbnn}
\begin{tabular}{lccccccc}
\toprule
Dataset & Method & 12.5\% & 25.0\% & 37.5\% & 50.0\% & 62.5\% & 75.0\% \\
\midrule
\multirow{2}{*}{Caltech101} 
& NBNN~\citep{boiman2008defense}   & 88.87 & 88.57 & 88.43 & 87.20 & 84.17 & 85.67 \\
& NA-MVP & \textbf{92.07} & \textbf{92.10} & \textbf{91.60} & \textbf{91.30} & \textbf{90.07} & \textbf{89.37} \\
\midrule
\multirow{2}{*}{OxfordPets} 
& NBNN~\citep{boiman2008defense}   & 87.47 & 86.00 & 85.53 & 83.07 & 82.50 & 80.67 \\
& NA-MVP & \textbf{88.50} & \textbf{88.40} & \textbf{88.23} & \textbf{88.13} & \textbf{86.93} & \textbf{86.23} \\
\bottomrule
\end{tabular}
\end{table}
\subsection{Parameter Study}
\label{C4}
\paragraph{Parameter Study of the Auxiliary Loss Weight \(\lambda_{\text{i}}\)}
We study the effectiveness of the auxiliary loss weight \(\lambda_{\text{i}}\), which controls the contribution of the ITBP loss during supervised training. As shown in Table~\ref{tab:lambda_study}, we evaluate \(\lambda_{\text{i}} \in \{0.01, 0.05, 0.1, 0.5\}\) across DTD, OxfordPets, and UCF101 under different noise levels. In particular, \(\lambda_{\text{i}} = 0.1\) consistently delivers the best or competitive results under different conditions. Therefore, we adopt \(\lambda_{\text{i}} = 0.1\) as the default setting in all experiments.

\paragraph{Parameter Study of the parameter $\theta$ in UOT}
To investigate the effect of the parameter $\theta$ in unbalanced OT, which regulates the mapping size of prompts on the feature map, we conducted additional experiments on the DTD dataset under varying noise rates and $\theta$ values ranging from 0.5 to 1.0. As shown in Table~\ref{tab:theta}, we observe that performance varies with $\theta$, and optimal results are typically achieved when $\theta$ is within the range of 0.8–0.9 across different noise levels.  This indicates that optimal alignment between multi-view prompts and the feature map is achieved when approximately 80\%–90\% of patch tokens are involved in the prompt interaction. Consequently, we adopt $\theta$ = 0.9 as the default setting in all our main experiments to ensure a good balance between sufficient prompt supervision and robustness under noise.
\begin{table}[t]
\centering
\setlength{\tabcolsep}{3.2pt}
\caption{Performance under different noise rates and $\theta$ values. (\%)}
\label{tab:theta}
\begin{tabular}{lcccccc}
\toprule
Noise rate/$\theta$ & 0.5 & 0.6 & 0.7 & 0.8 & 0.9 & 1.0 \\
\midrule
25.00\% & 61.87 & 62.83 & 63.30 & \textbf{63.80} & 63.13 & 63.37 \\
50.00\% & 57.57 & 58.73 & 58.07 & 58.67 & \textbf{58.80} & 58.30 \\
75.00\% & 47.43 & 48.30 & 47.67 & 47.13 & \textbf{48.63} & 46.30 \\
\bottomrule
\end{tabular}
\end{table}

\subsection{Additional Visual Analysis.}
\label{A:failure}

\begin{figure}[t]
  \centering
  % \fbox{\rule{0pt}{0.5in} \rule{0.9\linewidth}{0pt}}
  \includegraphics[width=1\linewidth]{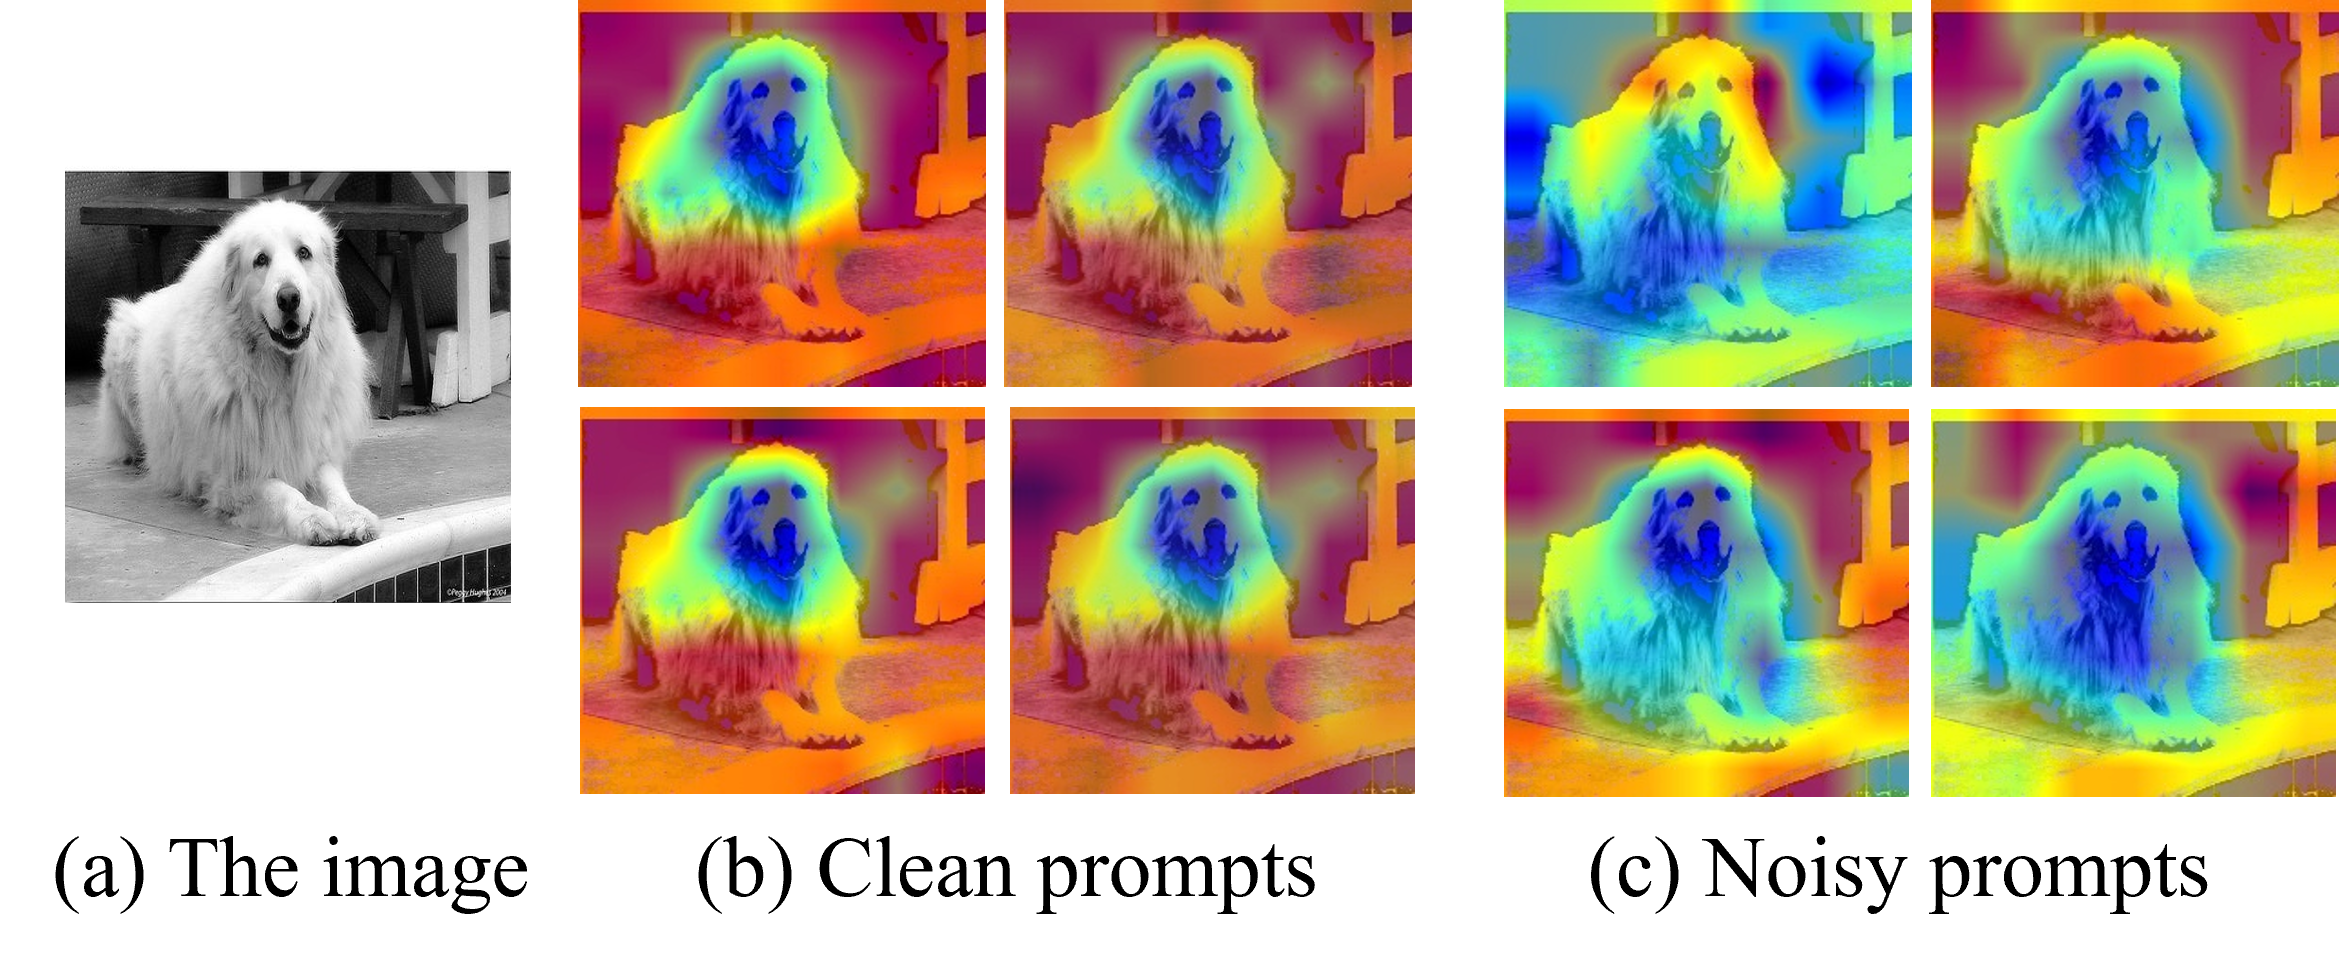}
   \caption{Visualizations for clean samples.}
   \label{fig:onecol}
   % \vspace{-15pt}
\end{figure}
To provide deeper insight into how our bi-directional multi-view prompts capture clean and noisy semantics, we visualize the learned attention maps under both clean and noisy samples. Figure \ref{fig:onecol} extends the transport maps from Fig. 4 to include representative clean samples, while Figure \ref{fig:single} illustrates failure cases on the OxfordPets dataset.

\paragraph{Successful Separation of Semantics} For noisy samples, noisy prompts focus on irrelevant regions such as background, while clean prompts consistently attend to meaningful object parts. In contrast, for clean samples , noisy prompts exhibit weak and unfocused alignment, indicating the absence of distinct noisy semantics. This clear contrast confirms that our bi-directional prompts effectively distinguish between clean and noisy signals. 

\paragraph{Analysis of Failure Cases} To better understand the limitations of our method, we further visualize failure cases on the OxfordPets dataset, as shown in Figure \ref{fig:single}. The figure illustrates attention maps of several learned clean and noisy prompts. We observe that in these cases the model fails to clearly distinguish between clean- and noise-oriented prompts. For example, the bottom-right clean prompt in (b2) and the bottom-right noisy prompt in (b3) exhibit highly similar activation patterns, indicating that the intended separation between clean and noisy supervision is not well preserved. Moreover, the heatmaps reveal that many prompts predominantly focus on background regions rather than the object of interest. This misalignment reduces the effectiveness of prompt-feature alignment, leading to incorrect label predictions. Such cases highlight that the current design may overfit spurious background cues when discriminative foreground signals are weak or ambiguous, suggesting the need for more flexible and accurate prompt learning mechanisms in future work.
\begin{figure*}[t]
    \centering
    \includegraphics[width=14cm]{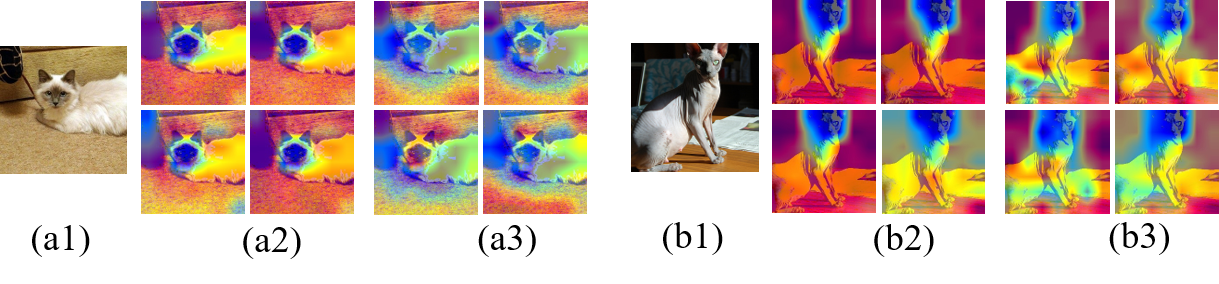}
    \caption{Visualization of failure cases on OxfordPets. (a1) \& (b1): The image; (a2) \& (b2): The learned multi-view clean prompts; (a3) \& (b3): The learned multi-view noisy prompts.}\label{fig:single}
    % \vspace{-15pt}
\end{figure*}
\subsection{Experiments on Waterbirds Dataset}
To further assess robustness, we conducted experiments on the Waterbirds dataset~\citep{sagawadistributionally} under multiple levels of label noise. The Waterbirds dataset is a common benchmark for studying spurious correlations, as its backgrounds (water or land) are strongly associated with class labels and often occupy a large portion of the image. This makes it suitable for evaluating sensitivity to background–foreground imbalance or noisy supervision. As shown in Table~\ref{tab:waterbirds}, accuracy decreases as the noise level increases, yet NA-MVP consistently outperforms NLPrompt across all settings. These results suggest that NA-MVP is relatively robust to mislabeled data and performs well on datasets with both small and large background regions, benefiting from its unbalanced optimal transport formulation, which enables the model to downweight irrelevant or misleading signals.
\begin{table}[t]
\centering
\setlength{\tabcolsep}{1.6pt}
\caption{Accuracy comparison on the Waterbirds dataset. (\%)}
\label{tab:waterbirds}
\begin{tabular}{lcccccc}
\toprule
Method/Noise rate & 12.5\% & 25\% & 37.5\% & 50\% & 62.5\% & 75\%  \\
\midrule
NLPrompt~\citep{pan2025nlprompt} & 74.23 & 72.47 & 71.50 & 68.43 & 64.80 & 58.27 \\
NA-MVP   & \textbf{75.27} & \textbf{74.40} & \textbf{72.07} & \textbf{69.27} & \textbf{65.47} & \textbf{59.23} \\
\bottomrule
\end{tabular}
\end{table}

\subsection{Generalization of NA-MVP }
To further demonstrate the generalization capability of our NA-MVP framework,  we apply it to two representative prompt-tuning methods beyond CoOp: VPT~\citep{jia2022visual} and MaPLe~\citep{khattak2023maple}. As shown in Table \ref{tab:VPT}, NA-MVP consistently improves their performance on the DTD dataset under various symmetric noise levels, demonstrating its strong generalization.
\begin{table}[t]
\centering
\setlength{\tabcolsep}{1.6pt}

\caption{The generalization of NA-MVP. }
\begin{tabular}{lcccccccc}
\toprule
Method/Noise rate & 12.5\% & 25\% & 37.5\% & 50\% & 62.5\% & 75\%  \\
\midrule
VPT~\citep{jia2022visual}         & 57.50 & 55.37 & 50.70 & 45.03 & 36.93 & 25.27 \\
\textbf{VPT+Ours}    & \textbf{68.43} & \textbf{66.93} & \textbf{66.10} & \textbf{63.57} & \textbf{60.00} & \textbf{53.80} \\
\midrule
MaPLe~\citep{khattak2023maple}       & 63.27 & 55.00 & 49.07 & 40.20 & 32.67 & 19.93 \\
\textbf{MaPLe+Ours}  & \textbf{69.70} & \textbf{67.50} & \textbf{65.37} & \textbf{62.83} & \textbf{56.47} & \textbf{45.83} \\
\bottomrule
\end{tabular}
\label{tab:VPT}
\end{table}
\subsection{Computation Cost and Parameter Analysis}
We compare the inference time of NA-MVP with the baseline method CoOp~\citep{zhou2022learning} and NLPrompt~\citep{pan2025nlprompt} on OxfordPets. As reported in Table~\ref{tab:cost}, NA-MVP achieves the fastest inference time of 5.778 seconds, surpassing CoOp by 25.2\% and NLPrompt by 79.6\%, demonstrating strong efficiency despite its multi-view design. Although training time increases, the gain remains practical given NA-MVP's consistent robustness across noise levels, offering a favorable trade-off between efficiency and performance.

Regarding model parameters, NA-MVP (N=4) uses 16,384 learnable parameters, slightly more than the baselines. However, performance gains stem from our bi-directional noise-aware design rather than parameter scale alone. This is further supported by NA-MVP’s consistent superiority even under matched parameter budgets (N=1), as shown in Figure \ref{fig:accuracy_noise} (Sec.~\ref{sec4.3}).
\begin{table}
  \centering
  \small  % 设置字体小一些
  \caption{Comparison of computational cost and model parameters.}
  \label{tab:cost}
  \setlength{\tabcolsep}{2.5pt} 
  \begin{tabular}{@{}lccc@{}}
    \toprule
    Settings & CoOp~\citep{zhou2022learning} & NLPrompt~\citep{pan2025nlprompt} & NA-MVP(N=4) \\ 
    \midrule
    Training Time (s) & 1.875 & 4.394 &6.285  \\ 
    Inference Time (s) & 7.719 & 28.276 & 5.778 \\ 
    Parameters & 8,192 & 8,192 & 16,384 \\ 
    \bottomrule
  \end{tabular}
  % \vspace{-10pt}
\end{table}

% \section{llm usage}
% Standard editing tools, including large language models, were used occasionally to polish the presentation of the manuscript (e.g., grammar, spelling, and word choice). Their use was limited to light language refinement, and they did not contribute to the conceptual development, methodology, experiments, or analysis of this work.
